# Supplementary material for: PlugSonic: a web- and mobile-based platform for binaural audio and sonic narratives
Source: arXiv:2008.04638 source file (2020-08-11)
Supplement: Supplementary file 1 [file appendix_A.tex]

\appendix{Appendix A - }
\textbf{PlugSonic Sample UI controls details}

\begin{figure*}[ht!]
	\centering
	\includegraphics[width=1\linewidth]{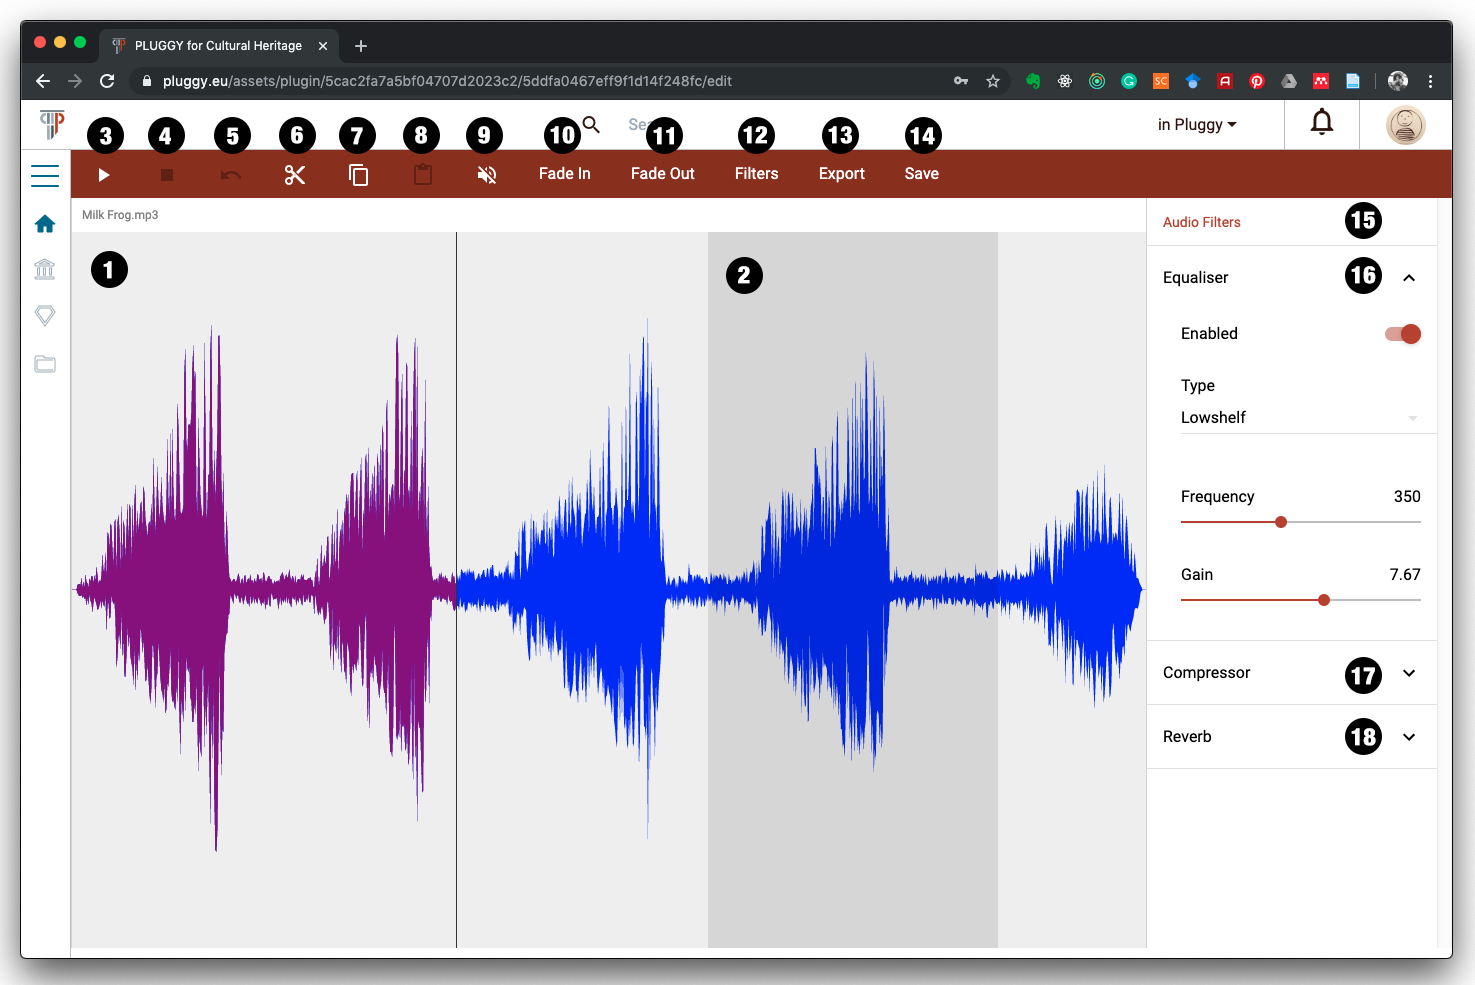}
	\caption{PlugSonic Sample User Interface}
    \label{fig:UI_Sample_appendix}
\end{figure*}

With reference to Figure \ref{fig:UI_Sample_appendix}, the user interface includes:
\begin{enumerate}
    \item Waveform of the audio file with filename on the top left corner
    \item Use of mouse to control the playback start and end points and select parts of the waveform to be modified
    \item Play button to reproduce the whole audio file or the selected part
    \item Stop button to stop reproduction
    \item Undo button to cancel edit actions
    \item Cut button to cut part of the waveform
    \item Copy button to copy part of the waveform
    \item Paste button to paste cut/copied part of the waveform
    \item Mute button to mute part of the waveform
    \item Fade In button to apply a volume fade in to the selection
    \item Fade Out button to apply a volume fade out to the selection
    \item Filters button to open the filters/effects menu (15)
    \item Export button to save the modified audio file to the users device
    \item Save button to save the modified audio file to the PLUGGY social platform
    \item Audio Filters/Effects menu
    \item Equaliser panel. Includes: lowpass, highpass, bandpass, lowshelf, highshelf, peaking and notch filters
    \item Compressor effect panel with threshold, knee, ratio, attack and release controls
    \item Reverb effect panel. Includes small, medium and large room reverbs
\end{enumerate}
