# Supplementary material for: PlugSonic: a web- and mobile-based platform for binaural audio and sonic narratives
Source: arXiv:2008.04638 source file (2020-08-11)
Supplement: Supplementary file 2 [file appendix_B.tex]

\appendix{Appendix B - }
\textbf{PlugSonic Soundscape Create UI controls details}

\begin{figure*}[ht!]
	\centering
	\includegraphics[width=1\linewidth]{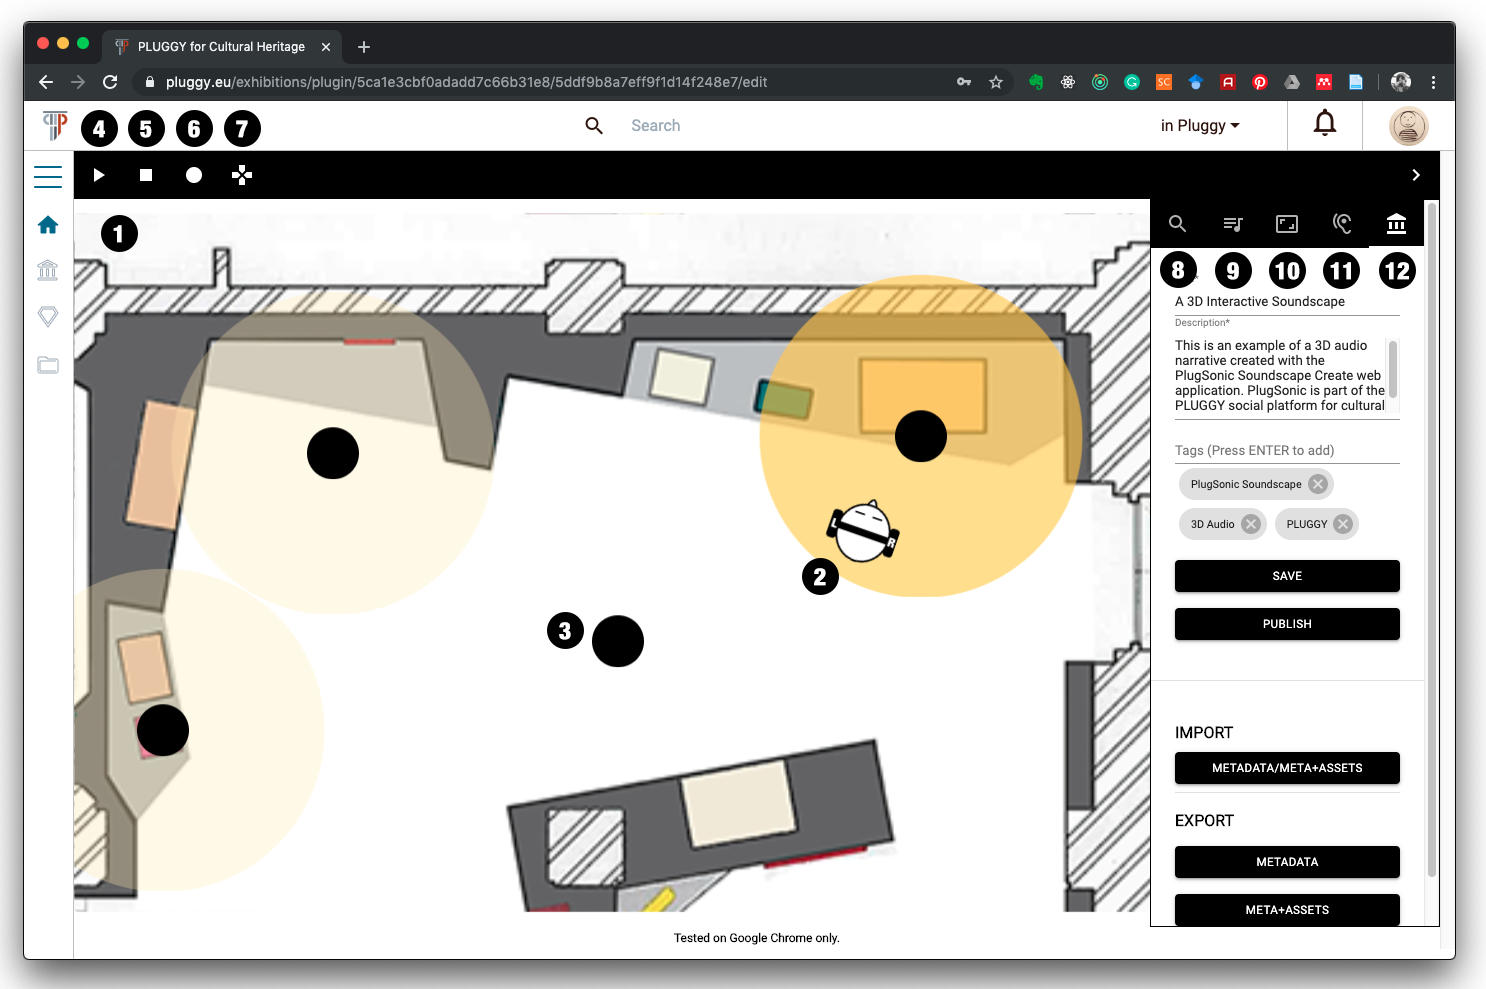}
	\caption{PlugSonic Soundscape Create User Interface}
    \label{fig:UI_Soundscape_appendix}
\end{figure*}

\begin{enumerate}
    \item Virtual room used for the curation of the soundscape
    \item Listener's icon representing position and orientation of the listener in the virtual environment
    \item Sound sources' icons representing position of each sound source in the virtual environment
    \item Play button
    \item Stop button
    \item Record button to record and export a .wav file of the rendered 3D audio
    \item Touch arrows button to open a panel showing touch arrow controls (necessary to navigate the soundscape on a touchscreen-based device)
    \item Search tab. To search and retrieve audio sources from the social platform (Figure \ref{fig:UI_Soundscape_MenuAll}.A):
        \begin{enumerate}[label=\alph*.]
            \item \textit{Search} text field
            \item Dropdown menu to search among the user's audio assets (\textit{My Assets}) or the whole social platform (\textit{All Pluggy})
            \item Dropdown menu to choose the ordering of the results
            \item \textit{Search} button
            \item One button for each sound found by the search. Upon clicking a button the source is retrieved and added to the soundscape.
        \end{enumerate}
    \item Sound sources' tab. Each sound source has the following options (Figure \ref{fig:UI_Soundscape_MenuAll}.B):
        \begin{enumerate}[label=\alph*.]
            \item \textit{On/off} toggle to activate/deactivate the sound
            \item \textit{Volume} slider
            \item Position options:
                \begin{enumerate}[label=\roman*.]
                    \item \textit{Relative to listener} toggle. To set the sound's position in an absolute or relative fashion
                    \item Position sliders. \textit{X/Y/Z} for absolute positioning or \textit{Angle/Distance} for relative positioning
                \end{enumerate}
            \item \textit{Loop} toggle to choose if the sound source will loop or play only once
            \item \textit{Spatialisation} toggle to turn on/off the spatialisation engine. When off the source is reproduced as a mono/stereo file depending on the original file format
            \item Reach options:
                \begin{enumerate}[label=\roman*.]
                    \item \textit{Reach} toggle - to turn on/off the interaction area. The interaction area (in yellow in Figure \ref{fig:UI_Soundscape_appendix}) is used to control the interaction between listener and sound source. When on, the listener will be able to hear the specific sound source only when they are inside the interaction area.
                    \item \textit{Reach radius} slider - to choose the size of the interaction area
                    \item \textit{Reach behaviour} dropdown menu - to choose the type of action the app will perform when entering/exiting the interaction area.
                        \begin{itemize}
                            \item \textit{Fade in and out} - playback will start as the user clicks the Play button but the source's volume will fade in/out as the listener enters/exits the interaction area
                            \item \textit{Start when entering} - Playback will start as the listener enters the interaction area
                        \end{itemize}
                    \item \textit{Fade duration} slider - to set the  volume's fade in/out duration
                \end{enumerate}
            \item \textit{Timings} dropdown menu - to set an order in the reproduction of the sound sources. The reproduction of a specific source can be constrained to the start of another one.
            \item \textit{Hidden} toggle - to hide the sound source in the Soundscape Experience apps so that the user cannot see the source's position on the screen
            \item \textit{Delete} button - to delete the sound source from the soundscape
        \end{enumerate}
    \item Room options tab. The room has the following options (Figure \ref{fig:UI_Soundscape_MenuAll}.C):
        \begin{enumerate}[label=\alph*.]
            \item \textit{Room Shape} dropdown menu (rectangular or round)
            \item \textit{Room Size} text fields (Width/Depth/Height)
            \item \textit{Room floorplan} - to search and select an image asset to be used as the soundscape's floor-plan.
            \item \textit{Reset listener position} button - to reset the listener's position to coordinate (0,0)
        \end{enumerate}
    \item Listener's options tab - to set options regarding the 3D audio rendering engine. The listener's options are the following (Figure \ref{fig:UI_Soundscape_MenuAll}.D):
        \begin{enumerate}[label=\alph*.]
            \item \textit{Performance mode} toggle. When on, the performance mode is enabled, requiring less computational effort, allowing the rendering on low performance devices.
            \item \textit{HRTF function} dropdown menu - to select the head related transfer functions to be used for the 3D sound rendering
            \item \textit{HRTF sample length} dropdown menu - to choose between 128/256/512 samples long HRTFs
        \end{enumerate}
    \item Exhibition tab - to set the exhibition’s options, save and publish the exhibition (Figure \ref{fig:UI_Soundscape_appendix}). It includes:
        \begin{enumerate}[label=\alph*.]
            \item \textit{Title} text field - to set the exhibition’s title
            \item \textit{Description} text field - to add a description of the soundscape
            \item \textit{Tags} text field and icons - to add/delete tags to the exhibition
            \item \textit{Save} button - to save the exhibition in the social platform
            \item \textit{Publish/Unpublish} button - to make the exhibition available or not to the social platform's users.
            \item \textit{Import} button - to import a previously exported soundscape in either format (metadata or metadata+assets)
            \item \textit{Export} metadata button - to export the exhibition’s metadata (will require access to PLUGGY social platform to retrieve the audio files)
            \item \textit{Export} metadata+assets button - to export the exhibition’s metadata and the audio assets in one file (will not require access to PLUGGY social platform to retrieve the audio files. Can be experienced when off-line)
        \end{enumerate}
\end{enumerate}
